# Supplementary material for: Deep Metric Learning with Chance Constraints
Source: arXiv:2209.09060 source file (2023-09-06)
Supplement: Supplementary file 1 [file appendix.tex]

\section{Proofs}
\label{app:proofs}
\subsection{Proof of Proposition 1}
\begin{proposition} \label{proposition1}
Given $N$ i.i.d. samples $\mathcal{D}=\lbrace (x_i, y_i)_i{\in}\mathcal{X}{\times}\mathcal{Y}\mid i{\in}\mathcal{N}\rbrace$ and a set $\mathcal{R}\subset\mathcal{N}$ of cardinality $M$, if $\ell^{\mathcal{R}}_\theta(r_i, x_j,y_{i,j})$ is $\zeta^\ell$-Lipschitz and bounded by $L$, $\mathcal{R}=\cup_c\mathcal{R}_c$ with $\mathcal{R}_c$ is the $\delta$-cover of the samples in class $c$, the conditional class distribution $p_{y_{i,j}\sim \lbrace 0,1\rbrace}(y=y^\prime\mid x_i, x_j)=\mu(y^\prime,x_i,x_j)$ is $\zeta^\mu$-Lipschitz, and zero training loss $\ell^{\mathcal{R}}_\theta(r_i, x_j,y_{i,j})=0,\, \forall (i,j)$; then we have at least $1-\gamma$ probability:
$$ \tfrac{1}{N^2}\textstyle\sum_{ij} \ell^{\mathcal{R}}_\theta(x_i, x_j,y_{i,j}) \leqslant \mathcal{O}(\delta) + \mathcal{O}(\sqrt{\tfrac{1}{N^2}})$$
\end{proposition}
\begin{proof}
We express $ \tfrac{1}{N^2}\textstyle\sum_{ij} \ell^{\mathcal{R}}_\theta(x_i, x_j,y_{i,j})$ as:
\begin{equation}\label{eq:putin}
\begin{split}
&\vert \tfrac{1}{N^2}\textstyle\sum_{ij} \ell^{\mathcal{R}}_\theta(x_i, x_j,y_{i,j}) \vert = \vert \tfrac{1}{N^2}\textstyle\sum_{ij} \ell^{\mathcal{R}}_\theta(x_i, x_j,y_{i,j}) - E_{x_i,x_j,y_{i,j}}[\ell^{\mathcal{R}}_\theta(x_i, x_j,y_{i,j})] + E_{x_i,x_j,y_{i,j}}[\ell^{\mathcal{R}}_\theta(x_i, x_j,y_{i,j})] \vert \\
&\leqslant \vert \tfrac{1}{N^2}\textstyle\sum_{ij} \ell^{\mathcal{R}}_\theta(x_i, x_j,y_{i,j}) - E_{x_i,x_j,y_{i,j}}[\ell^{\mathcal{R}}_\theta(x_i, x_j,y_{i,j})]\vert + \vert E_{x_i,x_j,y_{i,j}}[\ell^{\mathcal{R}}_\theta(x_i, x_j,y_{i,j})] \vert
\end{split}
\end{equation}
Now, using Hoeffding's Inequality, we can bound the first term with probability at least $1-\gamma$ as:
$$ \vert \tfrac{1}{N^2}\textstyle\sum_{ij} \ell^{\mathcal{R}}_\theta(x_i, x_j,y_{i,j}) - E_{x_i,x_j,y_{i,j}}[\ell^{\mathcal{R}}_\theta(x_i, x_j,y_{i,j})]\vert \leqslant \sqrt{\frac{L^2\log(\tfrac{1}{\gamma})}{2N^2}}$$
For  $\vert E_{x_i,x_j,y_{i,j}}[\ell^{\mathcal{R}}_\theta(x_i, x_j,y_{i,j})] \vert$ we consider conditional expectation for given $(x_i,x_j)$ in the dataset:
$$ E_{x_i,x_j,y_{i,j}}[\ell^{\mathcal{R}}_\theta(x_i, x_j,y_{i,j})] = E_{x_i,x_j}[E_{y_{i,j}}[\ell^{\mathcal{R}}_\theta(x_i, x_j,y_{i,j})]]$$
We express $E_{y_{i,j}}[\ell^{\mathcal{R}}_\theta(x_i, x_j,y_{i,j})]$ as:
$$ E_{y_{i,j}}[\ell^{\mathcal{R}}_\theta(x_i, x_j,y_{i,j})] = \sum_{k\in\lbrace0,1\rbrace}p_{y_{i,j}\sim \mu(y, x_i,x_j)}(y_{i,j}=k) \ell^{\mathcal{R}}_\theta(x_i, x_j,y_{i,j}) $$
We know that $\exists r_i\in\mathcal{R}$ such that $\Vert r_i - x_i\Vert \leqslant \delta$ form $\mathcal{R}$ being $\delta$-cover. Then we can write:
\begin{equation}
\nonumber
\begin{split}
p_{y_{i,j}\sim \mu(y, x_i,x_j)}(y_{i,j}=k)&= p_{y_{i,j}\sim \mu(k, x_i,x_j)}(y_{i,j}=k) + p_{y_{i,j}^\prime\sim \mu(y, r_i,x_j)}(y_{i,j}^\prime=k) -p_{y_{i,j}^\prime\sim \mu(y, r_i,x_j)}(y_{i,j}^\prime=k) \\
&\leqslant p_{y_{i,j}^\prime\sim \mu(y, r_i,x_j)}(y_{i,j}^\prime=k) + \vert p_{y_{i,j}\sim \mu(y, x_i,x_j)}(y_{i,j}=k) - p_{y_{i,j}^\prime\sim \mu(y, r_i,x_j)}(y_{i,j}^\prime=k)\vert \\
&\leqslant p_{y_{i,j}^\prime\sim \mu(y, r_i,x_j)}(y_{i,j}^\prime=k) + \vert \mu(k, x_i,x_j) - \mu(k, r_i,x_j)\vert
\end{split}
\end{equation}
Then $E_{y_{i,j}}[\ell^{\mathcal{R}}_\theta(x_i, x_j,y_{i,j})]$ can be bounded as:
\begin{equation}
\nonumber
\begin{split}
E_{y_{i,j}}[\ell^{\mathcal{R}}_\theta(x_i, x_j,y_{i,j})] &\leqslant
\sum_{k\in\lbrace0,1\rbrace}p_{y_{i,j}^\prime\sim \mu(y, x_i,x_j)}(y_{i,j}\prime=k) \ell^{\mathcal{R}}_\theta(x_i, x_j,y_{i,j}^\prime) \\
&+ \vert \mu(k, x_i,x_j) - \mu(k, r_i,x_j)\vert \ell^{\mathcal{R}}_\theta(x_i, x_j,y_{i,j}^\prime) \\
& \overset{(1)}{\leqslant} \sum_{k\in\lbrace0,1\rbrace}p_{y_{i,j}^\prime\sim \mu(y, x_i,x_j)}(y_{i,j}\prime=k) \ell^{\mathcal{R}}_\theta(x_i, x_j,y_{i,j}^\prime) + 2\zeta^{\mu}L\delta
\end{split}
\end{equation}
where in (1) we use $\zeta^{\mu}$-Lipschitz of density function, boundness of the loss and $\delta$-cover property. For the first term, we similarly express the loss, $\ell^{\mathcal{R}}_\theta(x_i, x_j,y_{i,j}^\prime)$, as:
\begin{equation}
\nonumber
\begin{split}
\ell^{\mathcal{R}}_\theta(x_i, x_j,y_{i,j}^\prime) &= \vert \ell^{\mathcal{R}}_\theta(x_i, x_j,y_{i,j}^\prime) + \ell^{\mathcal{R}}_\theta(r_i, x_j,y_{i,j}^\prime)  - \ell^{\mathcal{R}}_\theta(r_i, x_j,y_{i,j}^\prime)\vert \\
&\leqslant \ell^{\mathcal{R}}_\theta(r_i, x_j,y_{i,j}^\prime) + \vert \ell^{\mathcal{R}}_\theta(x_i, x_j,y_{i,j}^\prime) - \ell^{\mathcal{R}}_\theta(r_i, x_j,y_{i,j}^\prime)\vert \\
&\overset{(2)}{\leqslant} \ell^{\mathcal{R}}_\theta(r_i, x_j,y_{i,j}^\prime) + \zeta^\ell\delta
\end{split}
\end{equation}
where in (2) we use $\zeta^{\ell}$-Lipschitz of loss function and $\delta$-cover property. Finally, we bound $E_{y_{i,j}}[\ell^{\mathcal{R}}_\theta(x_i, x_j,y_{i,j})]$ as:
$$E_{y_{i,j}}[\ell^{\mathcal{R}}_\theta(x_i, x_j,y_{i,j})] \leqslant
\sum_{k\in\lbrace0,1\rbrace}p_{y_{i,j}^\prime\sim \mu(y, x_i,x_j)}(y_{i,j}\prime=k) \ell^{\mathcal{R}}_\theta(r_i, x_j,y_{i,j}^\prime) +\zeta^\ell\delta+ 2\zeta^{\mu}L\delta$$
The loss term of the right hand side of the inequality vanishes, since we assume zero training error. We finally obtain:
$$E_{y_{i,j}}[\ell^{\mathcal{R}}_\theta(x_i, x_j,y_{i,j})] \leqslant (\zeta^\ell+ 2\zeta^{\mu}L)\delta$$
Hence, we can bound the conditional expectation:
$$ E_{x_i,x_j}[E_{y_{i,j}}[\ell^{\mathcal{R}}_\theta(x_i, x_j,y_{i,j})]] \leqslant (\zeta^\ell+ 2\zeta^{\mu}L)\delta$$
Once we put back into the expression in \eqref{eq:putin}, we get with probability at least $1-\gamma$:
$$ \tfrac{1}{N^2}\textstyle\sum_{ij} \ell^{\mathcal{R}}_\theta(x_i, x_j,y_{i,j}) \leqslant (\zeta^\ell+ 2\zeta^{\mu}L)\delta + \sqrt{\frac{L^2\log(\tfrac{1}{\gamma})}{2N^2}}$$

\end{proof}
