# Supplementary material for: Deep Metric Learning with Chance Constraints
Source: arXiv:2209.09060 source file (2023-09-06)
Supplement: Supplementary file 2 [file table_conventional_all.tex]

\begin{table*}[!ht]
\centering
\caption{Comparison with the existing methods for the retrieval task in conventional experimental settings with BN-Inception and ResNet50 backbones where superscripts denote embedding size. Red: the best. Blue: the second best. Bold: previous SOTA.}
\label{tab:conventional}
%
% BNInception =========================================================
%
\begin{subtable}[t]{0.49\linewidth}
\centering
\caption{}
\label{tab:conventional_bninception}
\resizebox{\linewidth}{!}{%
\begin{tabular}{@{}ccccc@{}}
\toprule
\multicolumn{1}{l}{\textbf{Backbone $\rightarrow$}}     & \multicolumn{4}{c}{\textbf{BN-Inception-512D}}                                                                                                                \\ \midrule
\multicolumn{1}{l}{\textbf{Dataset $\rightarrow$}}      & \textbf{CUB}                          & \textbf{Cars196}                      & \textbf{SOP}                          & \textbf{In-shop}                      \\ \cmidrule(l){2-5} 
\multicolumn{1}{l}{\textbf{Method $\downarrow$}}        & \textbf{R@1}                          & \textbf{R@1}                          & \textbf{R@1}                          & \textbf{R@1}                          \\ \midrule
\multicolumn{1}{l|}{SoftTriple-L \cite{Qian_2019_ICCV}} & 65.40                                 & 84.50                                 & 78.60                                 & -                                     \\
\multicolumn{1}{l|}{C1-XBM-L \cite{wang2020cross}}      & 65.80                                 & 82.00                                 & 79.50                        & 89.90                                 \\
\multicolumn{1}{l|}{ProxyAnchor \cite{kim2020proxy}}    & 68.40                                 & 86.10 & 79.10                                 & \textbf{91.50}                        \\
\multicolumn{1}{l|}{DiVA \cite{milbich2020diva}}        & 66.80                                 & 84.10                                 & 78.10                                 & -                                     \\
\multicolumn{1}{l|}{ProxyFewer \cite{zhu2020fewer}}     & 66.60                                 & 85.50                                 & 78.00                                 & -                                     \\
\multicolumn{1}{l|}{Margin-S2SD \cite{roth2021s2sd}}    & \textbf{68.50}                        & {\color[HTML]{3166FF} \textbf{87.30}} & 79.30                                 & -                                     \\ 
\multicolumn{1}{l|}{HIST \cite{lim2022hypergraph}}    & {\color[HTML]{3166FF}\textbf{69.70}}                        & {\color[HTML]{FE0000} \textbf{87.40}} & \textbf{79.60}                                 & -                                     \\\midrule
\multicolumn{1}{l|}{C1-CCP-L}                           & 67.74                                 & 83.74                                 & {\color[HTML]{3166FF} \textbf{79.86}} & 90.98                                 \\
\multicolumn{1}{l|}{C2-CCP-L}                           & {\color[HTML]{FE0000} \textbf{69.87}} & 83.90                                 & {\color[HTML]{FE0000} \textbf{80.01}} & {\color[HTML]{3166FF} \textbf{91.72}} \\
\multicolumn{1}{l|}{MS-CCP-L}                                                & 69.09 & 86.01                                 & 79.75                                 & {\color[HTML]{FE0000} \textbf{91.84}} \\ \bottomrule
\end{tabular}%
}
\end{subtable}
%
% RESNET =========================================================
%
\begin{subtable}[t]{0.5\linewidth}
\centering
\caption{}
\label{tab:conventional_resnet}
\resizebox{\linewidth}{!}{%
\begin{tabular}{@{}ccccc@{}}
\toprule
\multicolumn{1}{l}{\textbf{Backbone $\rightarrow$}}                    & \multicolumn{4}{c}{\textbf{ResNet50}}                                                                                                                         \\ \midrule
\multicolumn{1}{l}{\textbf{Dataset $\rightarrow$}}                     & \textbf{CUB}                          & \textbf{Cars196}                      & \textbf{SOP}                          & \textbf{In-shop}                      \\ \cmidrule(l){2-5} 
\multicolumn{1}{l}{\textbf{Method $\downarrow$}}                       & \textbf{R@1}                          & \textbf{R@1}                          & \textbf{R@1}                          & \textbf{R@1}                          \\ \midrule
\multicolumn{1}{l|}{C1-XBM$^{128}$   \cite{wang2020cross}}             & -                                     & -                                     & 80.60                                 & 91.30                                 \\
\multicolumn{1}{l|}{ProxyAnchor$^{512}$ \cite{kim2020proxy}}           & 69.70                                 & 87.70                                 & 80.00\textsuperscript{$\dagger$} & 92.10\textsuperscript{$\dagger$} \\
\multicolumn{1}{l|}{DiVA$^{512}$ \cite{milbich2020diva}}               & 69.20                                 & {\color[HTML]{000000} 87.60}          & 79.60                                 & \textbf{-}                            \\
\multicolumn{1}{l|}{ProxyNCA++$^{512}$   \cite{teh2020proxynca++}}     & 66.30                                 & 85.40                                 & 80.20                                 & 88.60                                 \\
\multicolumn{1}{l|}{Margin-S2SD$^{512}$ \cite{roth2021s2sd}}           & 69.00                                 & {\color[HTML]{3166FF} \textbf{89.50}} & 81.20                                 & -                                     \\
\multicolumn{1}{l|}{LIBC$^{512}$ \cite{intrabatch}}                    & \textbf{70.30}                        & 88.10                                 & \textbf{81.40}                        & {\color[HTML]{FE0000} \textbf{92.80}} \\
\multicolumn{1}{l|}{ProxyAnchor-DIML$^{128}$   \cite{zhao2021towards}} & 66.46                                 & {\color[HTML]{000000} 86.13}          & 79.22                                 & -                                     \\

\multicolumn{1}{l|}{MS+Metrix$^{512}$ \cite{venkataramanan2022it}} & {\color[HTML]{FE0000} \textbf{71.40}} & {\color[HTML]{FE0000} \textbf{89.60}} & 81.00                                         &  92.20 \\
\multicolumn{1}{l|}{HIST$^{512}$ \cite{lim2022hypergraph}}    & {\color[HTML]{FE0000}\textbf{71.40}}                        & {\color[HTML]{FE0000} \textbf{89.60}} & \textbf{81.40}                                 & -                                     \\
\midrule
\multicolumn{1}{l|}{C1-CCP-L$^{512}$}                                  & 69.87                                 & 87.12                                 & {\color[HTML]{FE0000} \textbf{81.74}} & 92.07                                 \\
\multicolumn{1}{l|}{C2-CCP-L$^{512}$}                                  & {\color[HTML]{3166FF} \textbf{71.04}} & 85.93                                 & {\color[HTML]{3166FF} \textbf{81.66}} & {\color[HTML]{000000} 92.46}          \\
\multicolumn{1}{l|}{MS-CCP-L$^{512}$}                                  & {70.37} & {89.02} & 81.59                                 & {\color[HTML]{3166FF} \textbf{92.71}} \\ \bottomrule
\end{tabular}%
}
{\tiny\textsuperscript{$\dagger$}\textit{Results obtained from LIBC} \cite{intrabatch}.}
\end{subtable}
\end{table*}
